# Supplementary material for: KNN-DBSCAN: a DBSCAN in high dimensions
Source: arXiv:2009.04552 source file (2024-09-11)
Supplement: Supplementary file 2 [file pseudocode.tex]

\section{Pseudocode}\label{sec:pseudo}

\Cref{alg:local_mst} presents the pseudocode for \textsc{ParallelLocalMST}. \Cref{alg:findmin} presents the pseudocode for \textsc{FindMin} (Line 10 in \Cref{alg:local_mst}). Pseudocode of \textsc{DistributedCutMST} is shown in \Cref{alg:cut_mst}.

%%%%alg:local mst
\begin{algorithm}[h]
\small
\caption{Parallel local MST} \label{alg:local_mst}
\begin{spacing}{1.2}
\begin{algorithmic}[1]
    \Require graph $\mathbf{G}$, core points $\mathcal{I}_{\text{core}}$, labels $R$
    \Ensure labels $R$, cut edges $E_{\text{cut}}$, subtrees $\mathcal{T}$
\Procedure{ParallelLocalMST}{$\mathbf{G}, \mathcal{I}_{\text{core}}, \,R$}
    \State $\mathcal{T}\gets \mathcal{I}_{\text{core}}$, $E_{\text{cut}}\gets \emptyset$
    \State $L[i]\gets 1$, $i \in \mathcal{I}_{\text{core}}$ \Comment{initialize neighbor (edge) NO. to check}
    \Do
\LineComment{Find minimum edges}
    \State $ E_{\text{min}}[u]\gets \{u, -1, \text{sentinel}\}$, $u \in \mathcal{T}$
    \ForEach{point $i\in \mathcal{I}_{\text{core}}$}{\textbf{ in parallel}}
        \Do
        \State $e \gets \mathbf{G}[i,L[i]]$
        \State $ifbreak$ = \textsc{Findmin}($e, E_{\text{min}}, E_{\text{cut}}, R, L[i]$)
        \doWhile{($L[i] \leq M$) $\wedge$ ($ifbreak$)}
    \EndFor
    
\LineComment{Break symmetry}
    \State $R_{\mathcal{T}}[u]\gets E_{\text{min}}[u].j,\, u\in \mathcal{T}$ \Comment{initialize subtrees' roots}
    \ForEach{subtree $u\in \mathcal{T}$}{\textbf{ in parallel}}
        \State $v \gets R_{\mathcal{T}}[u]$
    \If{($v = -1$) $\vee$ ($u = R_{\mathcal{T}}[v] \wedge u < v$)}
        \State $R_{\mathcal{T}}[u]\gets u$
    \EndIf
    \EndFor
\LineComment{Pointer jumping}
    \State $Flags[u] \gets 1$, $u\in \mathcal{T}$ 
    \Do
        \ForEach{subtree $u\in \mathcal{T}$}{\textbf{ in parallel}}
            \If{$R_{\mathcal{T}}[u] \neq R_{\mathcal{T}}[R_{\mathcal{T}}[u]] $}
                \State $R_{\mathcal{T}}[u]\gets R_{\mathcal{T}}[R_{\mathcal{T}}[u]]$
            \ElsIf{$Flags[u]>0$} 
                \State $Flags[u] = 0$ \Comment{root for $u$ is found}
            \EndIf
        \EndFor    
    \doWhile{$\sum_u Flags[u]$ is changed}

\LineComment{Break cycles if cycle exits}
    \If{$\sum_u Flags[u] > 0$}
        \State \textsc{breakCycles}($\mathcal{T}, \,Flags,\, E_{\text{min}},\, R_{\mathcal{T}}$)
    \EndIf 
\LineComment{Update labels $R$ and subtree list $\mathcal{T}$}
    \State $N_{\mathcal{T}}^{\text{old}}\gets | \mathcal{T}|$, $\mathcal{T} \gets \emptyset$
        \State  $R[i] \gets R_{\mathcal{T}}[R[i]]$, $\mathcal{T} \gets \mathcal{T}\cup \{R[i] \}$, $i\in\mathcal{I}_\text{core}$
    \doWhile{$|\mathcal{T}| < N_{\mathcal{T}}^{\text{old}}$}
    \State \Return $R,\, E_{\text{cut}},\, \mathcal{T}$
\EndProcedure
\end{algorithmic}
\end{spacing}
\end{algorithm}

%%%%%% min edges
\begin{algorithm}[h]
\small
    \caption{Find minimum edges}\label{alg:findmin}
\begin{spacing}{1.2}
\begin{algorithmic}[1]
\Procedure{Findmin}{$e, E_{\text{min}}, E_{\text{cut}}, R, l$}
        \State $i \gets e.i$, $j \gets e.j$
        \If{$j$ lies in another process}
            \State $E_{\text{cut}}\gets E_{\text{cut}}\cup \{e\}$, $l\gets l+1$
        \ElsIf{$R[j] \neq -1$ and $R[j]\neq R[i]$}
            \State \textsc{pwrite}($E_{\text{min}}[R[i]], \, e$)
            \State \Return true
        \Else
            \State $l \gets l +1$
        \EndIf
        \State \Return false
\EndProcedure
\Procedure{pwrite}{$e_{\text{min}}, \, e$}
    \Do
        \State $w_{\text{old}}$ $\gets e_{\text{min}}.w$
    \doWhile{($e.w < w_{\text{old}}$) $\wedge$ (\textsc{LockFreeCAS}($e_{\text{min}}, w_{\text{old}}, e$))}
\EndProcedure
\Procedure{LockFreeCAS}{$e_{\text{min}}, w_{\text{old}}, e$}
    \If{$e_{\text{min}}.w = w_{\text{old}}$}
        \State $e_{\text{min}} \gets e$
        \State \Return true
    \Else
        \State \Return false
    \EndIf
\EndProcedure
\end{algorithmic}
\end{spacing}
\end{algorithm}

%%%%alg:cut mst
\begin{algorithm}[h]
\small
    \caption{Distributed cut MST} \label{alg:cut_mst}
%    \hspace*{\algorithmicindent} \textbf{Input:} labels $R$, cut edges $E_{\text{cut}}$, local subtrees $\mathcal{T}$\\
%    \hspace*{\algorithmicindent} \textbf{Output:} labels $R$
\begin{spacing}{1.2}
\begin{algorithmic}[1]
\Procedure{DistributedCutMST}{$E_{\text{cut}}, \,R,\, \mathcal{T}$}
\LineComment{Update cut edges}
        \ForEach{edge $e \in E_{\text{cut}}$}{\textbf{ in parallel}}
            \State $e.i \gets R[e.i]$
            \State update $e.j$ to label of $e.j$ \Comment{all to all exchange labels}
        \EndFor  
    \LineComment{Boruvka's iterations}
    \State $R_{\mathcal{T}}[u] \gets u,\, u\in \mathcal{T}$ 
    \State $\widehat{\mathcal{T}}\gets \mathcal{T}$, $\widehat{\mathcal{T}}_{l} \gets \mathcal{T}$, $N_{\text{root}}\gets$ MPI\_Allreduce($|\widehat{\mathcal{T}}_{l} |$)
    \Do
\LineComment{Find \textit{local} minimum cut edges $E_{\text{min}}^l$}
        \State $E_{\text{min}}^l[u]\gets \{u, -1, \text{sentinel}\}$, $u \in \widehat{\mathcal{T}}$
        \ForEach{edge $e \in E_{\text{cut}}$}{\textbf{ in parallel}}
            \If{$e.j \neq -1$} \Comment{only check active cut edge}
                \State \textsc{pwrite}($E_{\text{min}}^l[e.i], \, e$)
            \EndIf
        \EndFor          
\LineComment{Find \textit{global} minimum cut edges $E_{\text{min}}^g$}
        \State $E_{\text{recv}}\gets$ MPI\_Alltoallv($E_{\text{min}}^l$)
        \State $E_{\text{min}}^g[r]\gets \{r, -1, \text{sentinel}\}$, $r \in \widehat{\mathcal{T}}_{l}$
        \ForEach{edge $e \in E_{\text{recv}}$}{\textbf{ in parallel}}
                \State \textsc{pwrite}($E_{\text{min}}^g[e.i], \, e$)
        \EndFor          
\LineComment{Find roots of $\widehat{\mathcal{T}}_{l}$ and store in $R_l$}
        \State $R_l[r]\gets E_{\text{min}}^g[r].j$, $r \in \widehat{\mathcal{T}}_{l}$
        \State $R_l=$ \textsc{DistributedFindRoots}($R_l,\,\widehat{\mathcal{T}}_{l}$)
\LineComment{Update roots and cut edges}
        \State $\widehat{\mathcal{T}}\gets \emptyset$, $\widehat{\mathcal{T}}_{l}\gets \emptyset$, $N_{\text{root}}^\text{old}\gets N_{\text{root}}$
        \State $R_{\text{all}} \gets$ MPI\_Allgatherv($R_l$)
        \ForEach{subtree $u \in \mathcal{T}$}{\textbf{ in parallel}}
                \State $r \gets R_{\text{all}}[R_\mathcal{T}[u]]$, $R_\mathcal{T}[u] \gets r$, $\widehat{\mathcal{T}}\gets \widehat{\mathcal{T}}\cup \{r \}$
                \If{$r$ lies in local process}
                    \State $\widehat{\mathcal{T}}_{l} \gets \widehat{\mathcal{T}}_{l} \cup \{ r\}$
                \EndIf
        \EndFor 
        \State $N_{\text{root}}\gets$ MPI\_Allreduce($|\widehat{\mathcal{T}}_{l} |$)
        \ForEach{edge $e \in E_{\text{cut}}$}{\textbf{ in parallel}}
            \State $e.i \gets R_\text{all}[e.i]$, $e.j \gets R_\text{all}[e.j]$
            \If{$e.i = e.j$}
                \State $e.j = -1$ \Comment{edge becomes inactive}
            \EndIf
        \EndFor
    \doWhile{$N_\text{root} < N_{\text{root}}^\text{old} $ }
        \State $R[i] \gets R_{\mathcal{T}}[R[i]]$, $i\in \mathcal{I}_\text{core}$ \Comment{update core point's label}
    \State \Return $R$
\EndProcedure
\end{algorithmic}
\end{spacing}
\end{algorithm}
